# Supplementary material for: Minimalistic Collective Perception with Imperfect Sensors
Source: arXiv:2209.12858 source file (2023-09-01)
Supplement: Supplementary file 1 [file appendix_static_results.tex]

\appendix[Additional Results]
